# Supplementary material for: Hierarchy of exact low-dimensional reductions for populations of coupled oscillators
Source: arXiv:2108.10143 ancillary file (2022-02-01)
Supplement: Supplementary file 1 [file supplemental.pdf]

# Hierarchy of Exact Low-Dimensional Reductions for Populations of Coupled Oscillators
# Supplemental Material

Rok Cestnik and Arkady Pikovsky
*Department of Physics and Astronomy, University of Potsdam,*
*Karl-Liebknecht-Strasse 24/25, 14476, Potsdam-Golm, Germany*[*]

### Deriving kinetic equations for Ansatz 2

The kinetic equations in terms of moments read:

$$\frac{1}{n}\dot{Z}_n = \mathrm{i}\omega Z_n + hZ_{n-1} - h^* Z_{n+1} \ , \quad n \geq 1 \ . \tag{S1}$$

Within Ansatz 2 the moments $Z_n$ and variables $\beta_r$ are related via a binomial transform:

$$Z_n = \sum_{r=0}^{n} \binom{n}{r} \beta_r Q^{n-r} \ , \tag{S2}$$

whose inverse is:

$$\beta_r = \sum_{n=0}^{r} \binom{r}{n} Z_n (-Q)^{r-n} \ . \tag{S3}$$

The kinetic equations for $\beta_r$ variables can be obtained by deriving (S3) in time, inserting expressions for $\dot{Z}_n$ using (S1), expressing moments with $\beta_r$ variables using (S2), and assuming the OA equation for $Q$:

$$\dot{Q} = \mathrm{i}\omega Q + h - h^* Q^2. \tag{S4}$$

This yields Eqs. (12) in the main text:

$$\frac{1}{r}\dot{\beta}_r = \mathrm{i}\omega \beta_r - 2h^* Q\beta_r - h^* \beta_{r+1} \ , \quad r \geq 1 \ . \tag{S5}$$

We also sketch below the main steps of the reverse calculation: showing that (S4) and (S5) represent dynamics (S1). The first step involves calculating the derivative of $Z_n$ using (S2), (S4), (S5):

$$\dot{Z}_n = \sum_{r=0}^{n} \binom{n}{r} \left[\dot{\beta}_r Q^{n-r} + (n-r)\beta_r Q^{n-1-r}\dot{Q}\right] =$$

$$= \sum_{r=0}^{n} \binom{n}{r} \left[r\,(\mathrm{i}\omega\beta_r - 2h^* Q\beta_r - h^*\beta_{r+1})Q^{n-r} + (n-r)(\mathrm{i}\omega Q + h - h^* Q^2)\beta_r Q^{n-1-r}\right] =$$

$$= \sum_{r=0}^{n} \frac{n!}{r!(n-r)!} \Big[\mathrm{i}\omega\, n\, \beta_r Q^{n-r} + h\,(n-r)\beta_r Q^{n-1-r} - h^*\big((n+r)\beta_r Q^{n+1-r} + r\beta_{r+1}Q^{n-r}\big)\Big] =$$

$$= \mathrm{i}\omega\, n \sum_{r=0}^{n} \frac{n!}{r!(n-r)!}\beta_r Q^{n-r} + h\, n \sum_{r=0}^{n} \frac{(n-1)!}{r!(n-1-r)!}\beta_r Q^{n-1-r} - h^* \sum_{r=0}^{n} \frac{n!}{r!(n-r)!}\left((n+r)\beta_r Q^{n+1-r} + r\beta_{r+1}Q^{n-r}\right)$$

In the last expression one can easily identify the first term as $n\,\mathrm{i}\omega Z_n$ and the second term as $n\,hZ_{n-1}$. The third term $-n\,h^* Z_{n+1}$ requires more work:

$$\sum_{r=0}^{n} \frac{n!}{r!(n-r)!}\left((n+r)\beta_r Q^{n+1-r} + r\beta_{r+1}Q^{n-r}\right) =$$

$$= \sum_{r=0}^{n} \frac{n!}{r!(n+1-r)!}(n+1-r)(n+r)\beta_r Q^{n+1-r} + \sum_{r=1}^{n+1} \frac{n!}{r!(n+1-r)!} r(r-1)\beta_r Q^{n+1-r} =$$

$$= n \sum_{r=0}^{n+1} \frac{(n+1)!}{r!(n+1-r)!}\beta_r Q^{n+1-r} = n\, Z_{n+1}$$

Thus showing that (S2), (S4), (S5) indeed fulfill Eqs. (S1).

**Relating $Q_m, \beta_{r,m}$ variables to circular cumulants**

Recently, circular cumulants have been introduced to describe the vicinity of the OA manifold [1, 2]. These cumulants $\varkappa_n$ are defined by the following relation involving the moment EGF $F$:

$$\sum_{n=1}^{\infty} \varkappa_n k^n \equiv k \, \frac{\partial}{\partial k} \log(F) \, . \tag{S6}$$

The first cumulant therefore corresponds to the first moment, while the $n^{\text{th}}$ cumulant is a combination of the first $n$ moments, see first few expressions below:

$$\begin{aligned}
\varkappa_1 &= Z_1 & Z_1 &= \varkappa_1 \\
\varkappa_2 &= Z_2 - Z_1^2 & Z_2 &= \varkappa_2 + \varkappa_1^2 \\
\varkappa_3 &= \frac{1}{2}\left(Z_3 - 3Z_1Z_2 + 2Z_1^3\right) & Z_3 &= 2\varkappa_3 + 3\varkappa_1\varkappa_2 + \varkappa_1^3 \\
\varkappa_4 &= \frac{1}{6}\left(Z_4 - 4Z_1Z_3 - 3Z_2^2 + 12Z_1^2Z_2 - 6Z_1^4\right) & Z_4 &= 6\varkappa_4 + 8\varkappa_1\varkappa_3 + 3\varkappa_2^2 + 6\varkappa_1^2\varkappa_2 + \varkappa_1^4 \\
&\vdots & &\vdots
\end{aligned}$$

Similarly to our introduced variables $\beta_{r,m}$, on the OA manifold all the cumulants (except $\varkappa_1$) are equal to zero: $\varkappa_{n>1} = 0$.

Previously in [2], an extension of the OA manifold has been considered in the form of odd cumulants (except $\varkappa_1$) being zero and, the even ones proportional to powers of $\varkappa_2$: $\varkappa_{2n+1} = 0$, $\varkappa_{2n} = c_n \varkappa_2^n$. This case corresponds to two non-zero real-valued $\beta_{0,1}, \beta_{0,2} \in \mathbb{R}$ variables, and thus a superposition of two WCLDs.

A different special case has an even neater representation with circular cumulants. For $M = 1$, within the $Q, \beta_r$ representation of Ansatz 2, the lowest-order manifold beyond OA corresponds to two non-zero complex variables $Q$ and $\beta_1 \equiv \beta$, and a generating function of the form

$$F(k) = e^{kQ}(1 + \beta k). \tag{S7}$$

Substituting this into (S6) we obtain

$$\varkappa_1 = Q + \beta, \quad \varkappa_{n\geq 2} = (-1)^{n-1}\beta^n \, , \tag{S8}$$

and therefore this expanded manifold corresponds to a power-series hierarchy in cumulants:

$$\varkappa_{n\geq 2} = -(-\varkappa_2)^{n/2} \, , \tag{S9}$$

reminiscent to how OA corresponds to a power-series in moments: $Z_n = Z_1^n$.

### Expressions for elemental phase density contributions $P_{r,m}$ using only real quantities

In the main text, (19) gives the general expression for the elemental contributions $P_{r,m}$ in terms of the complex variables $Q_m$ and $\beta_{r,m}$. Here we give an expression using only real quantities $|Q_m|, |\beta_{r,m}|, \arg Q_m$ and $\arg \beta_{r,m}$:

$$P_{r,m}(\varphi) = \frac{|\beta_{r,m}|}{\pi} \frac{\sum_{n=0}^{r+1} \binom{r+1}{n} (-|Q_m|)^{r+1-n} \cos((1-n)\varphi - (r+1-n)\arg Q_m + \arg \beta_{r,m})}{(1 - 2|Q_m|\cos(\varphi - \arg Q_m) + |Q_m|^2)^{r+1}} \, . \tag{S10}$$

Note that only index $r$ is relevant to the density expression, index $m$ plays no role. Examples of $P_{r,m}$ contributions are depicted in Figure S1.

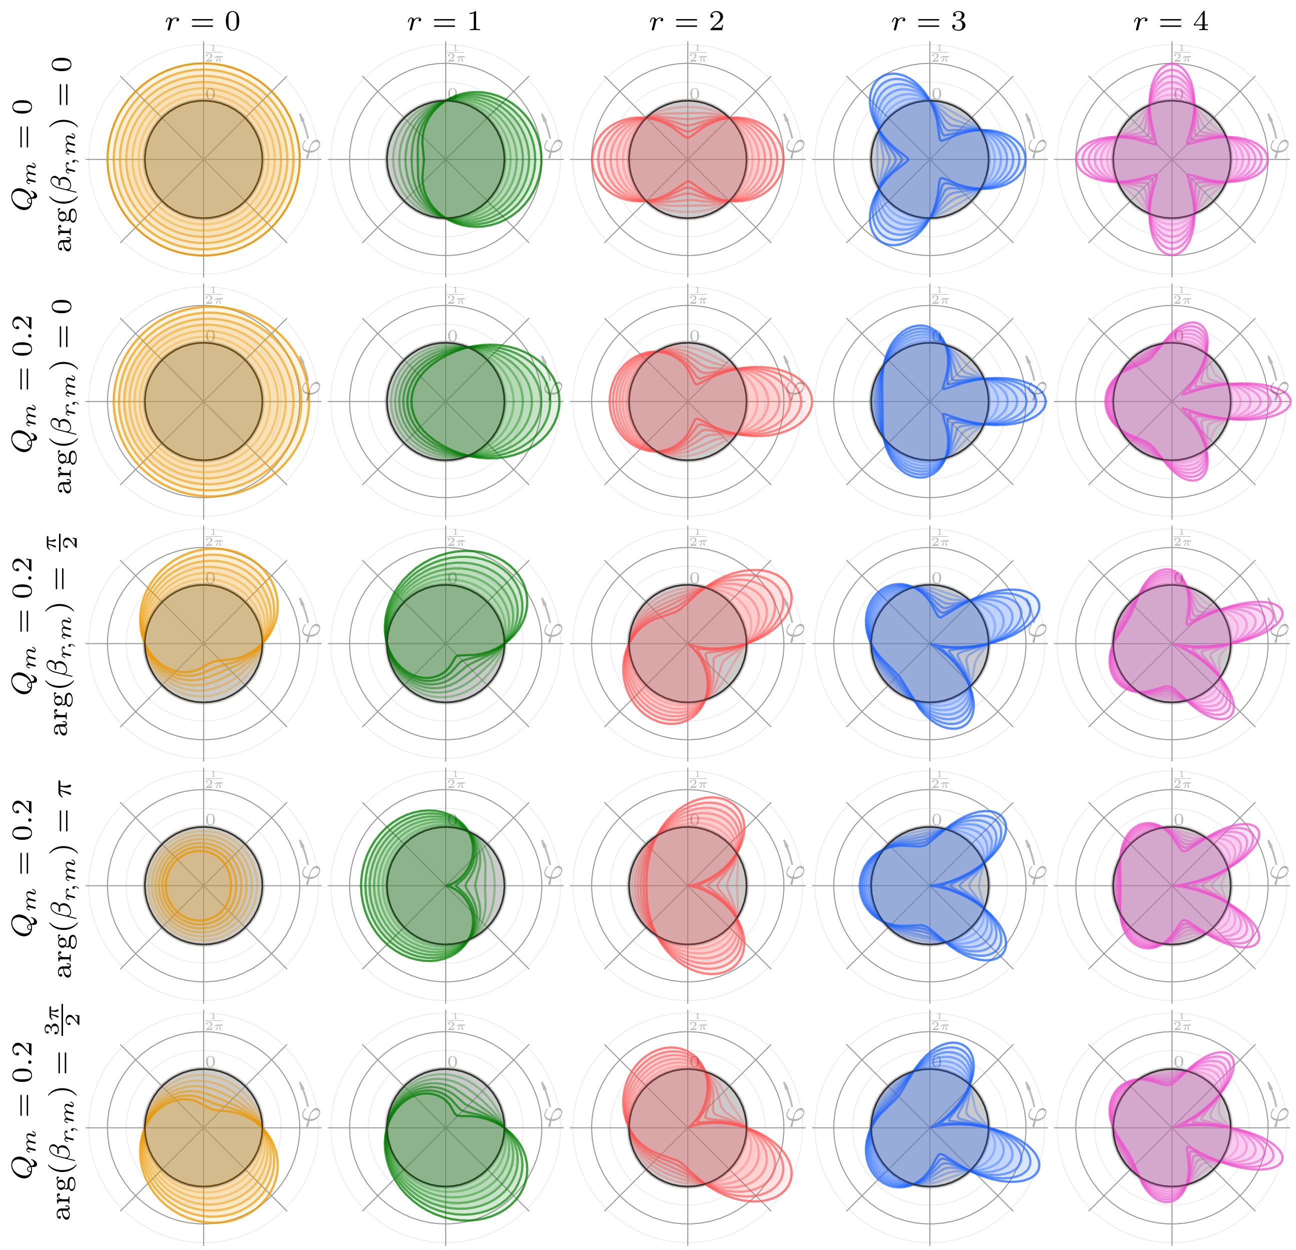


FIG. S1. Examples of elemental density contributions $P_{r,m}(\varphi)$ (S10), depicted in polar coordinates. First row entries corresponding to $Q_m = 0$ are exactly Fourier harmonics. The first column entries correspond to $r = 0$ contributions, which bare the normalization and thus, in general have non-zero mean (both positive or negative); in first row a uniform distribution, in second row an example of an offset WCLD which (for full density) corresponds to the OA manifold, in third row an example KJD with $\beta_{0,m}$ purely imaginary (mean zero), and in fourth row again offset WCLD but this time with negative mean. In each subplot, the different curves represent different absolute values of the corresponding variable $|\beta_{r,m}|$. Bold black circle represents zero and the gray disc inside holds negative values. Thin outer circle marks the $\frac{1}{2\pi}$ value, representing a uniform normalized distribution for reference.

### Distribution non-negativity restrictions on a set of $Q_m, \beta_{r,m}$ variables

It is not clear how to generally express the restrictions on state variables $Q_m, \beta_{r,m}$ imposed by the non-negative density condition. In practice one just has to check whether the complete sum is non-negative at every phase. However, for special simplified cases we can procure explicit conditions, and here we present them for two cases:

- $M = 1$ and $R_1 = 1$, with only 2 variables: $Q_1$ and $\beta_{1,1}$, we omit the indexes and denote them as $Q, \beta$. The conditions of non-negativity then read:

$$|Q| < 1, \qquad |\beta| \le \frac{1}{2}(1 - |Q|^2) \, . \tag{S11}$$

- A single KJD [3], realized as $M = 2$, $R_1 = R_2 = 0$, $\beta_{0,1} + \beta_{0,2} = 1$ and $Q_1 = 0$ is not invariant under evolution, but nevertheless can represent a physical state at a given point in time (e.g. can be used as an initial condition). In our formulation it has two parameters $Q_2$ and $\beta_{0,2}$ which we here denote without indexes. From their publication [3], Theorem 1 gives the non-negativity conditions:

$$|Q| < 1, \qquad |Q\beta| < 1, \qquad |Q\beta| - |Q|^2 \, \mathrm{Re}[\beta] \le \frac{1}{2}(1 - |Q|^2) \, . \tag{S12}$$

### Simulation of a finite ensemble of Josephson junctions

Here in Figure S2 we present numerical simulations of a finite ensemble of Josephson junctions

$$\dot{\varphi}_n = 1 + a \sin(\varphi_n) + \frac{\epsilon}{N} \sum_{m=1}^{N} \sin(\varphi_m) \, , \tag{S13}$$

for $a = 1.5$, $\epsilon = -0.7$ and two values of ensemble size $N$.

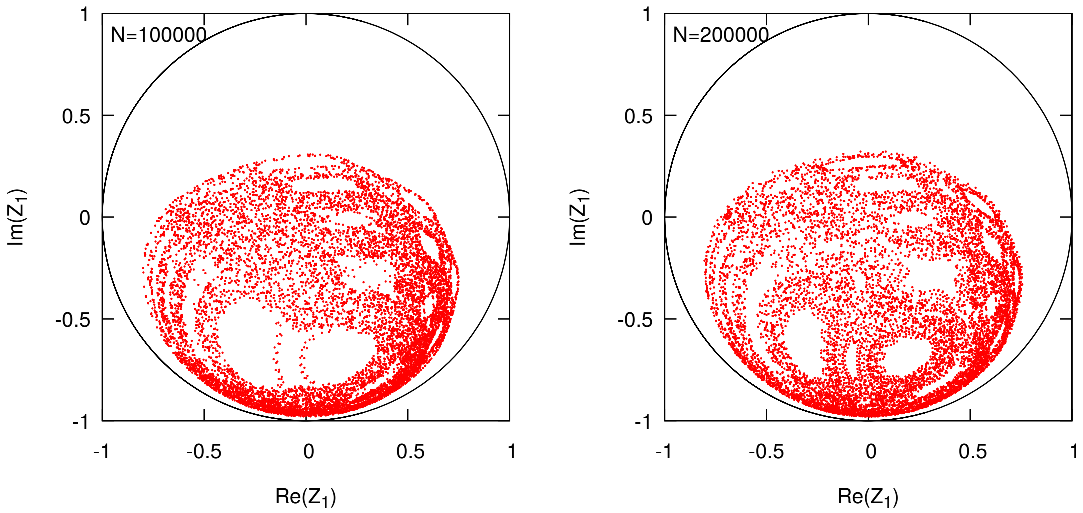


FIG. S2. Poincaré maps obtained from the simulations of (S13) under the same conditions as Figure 2 in the main text. Parameter values are $a = 1.5$, $\epsilon = -0.7$ and the initial condition $Z_1(t = 0) = 0.4$, $Z_{n>1}(t = 0) = 0$. The section is made according to the condition $\arg(\beta) = \pi$, $\frac{d}{dt}\arg(\beta) > 0$.

### Quasiperiodic dynamics of a two-population chimera

We consider a system of two coupled oscillatory populations with identical frequencies and distinct coupling strengths for intra- and interpopulation coupling:

$$\begin{aligned}\dot{\varphi}_n &= \omega + \frac{1+A}{2N}\sum_{m=1}^{N}\sin(\varphi_m-\varphi_n-\alpha) + \frac{1-A}{2N}\sum_{m=1}^{N}\sin(\psi_m-\varphi_n-\alpha)\ ,\\ \dot{\psi}_n &= \omega + \frac{1+A}{2N}\sum_{m=1}^{N}\sin(\psi_m-\psi_n-\alpha) + \frac{1-A}{2N}\sum_{m=1}^{N}\sin(\varphi_m-\psi_n-\alpha)\ ,\end{aligned} \tag{S14}$$

where $N$ represents the size of each population, $\alpha$ the coupling phase shift and $A$ the asymmetry of intra- and interpopulational interactions. This is a well studied system [4, 5], and was used to showcase the approaches of [1] and [2] as well. In the thermodynamic limit $N \to \infty$, the system displays a locally stable chimera state with one population fully synchronized, while the other remains partially synchronized. For general initial conditions the dynamics are quasiperiodic, while on the OA manifold (which is known for such populations of identical oscillators to be only neutrally stable [6]) they are periodic.

We now show that the dynamics on the simplest extended manifold of Ansatz 2, i.e. two variables $Q$ and $\beta_1 \equiv \beta$, can capture quasiperiodic behavior as well. The dynamical equations are written with $Q, \beta$ for one population and the corresponding variables $W, \eta$ for the other:

$$\begin{aligned}\dot{Q} &= h - h^*Q^2\ , & \dot{W} &= f - f^*W^2\ ,\\ \dot{\beta} &= -2h^*Q\beta\ , & \dot{\eta} &= -2f^*W\eta\ .\end{aligned} \tag{S15}$$

Here the coupling forces are $h = \frac{1}{4}\Big[(1+A)Z + (1-A)Y\Big]e^{-\mathrm{i}\alpha}$ and $f = \frac{1}{4}\Big[(1+A)Y + (1-A)Z\Big]e^{-\mathrm{i}\alpha}$ and we denoted the first moments of both populations with $Z = Q + \beta$ and $Y = W + \eta$. The frequency $\omega$ can be without loss of generality omitted by moving in the rotating reference frame. The simulation of Eqs. (S15) compared with a simulation on the OA manifold is shown in Figure S3. During the evolution, the second population fully synchronizes $|W| \to 1$, $\eta \to 0$ while the first remains partially synchronous ($|Z| < 1$, $\beta$ finite). The total dynamics are quasiperiodic with two incommensurate frequencies, as follows also from the application of the Watanabe-Strogatz theory [7] to this model [5].

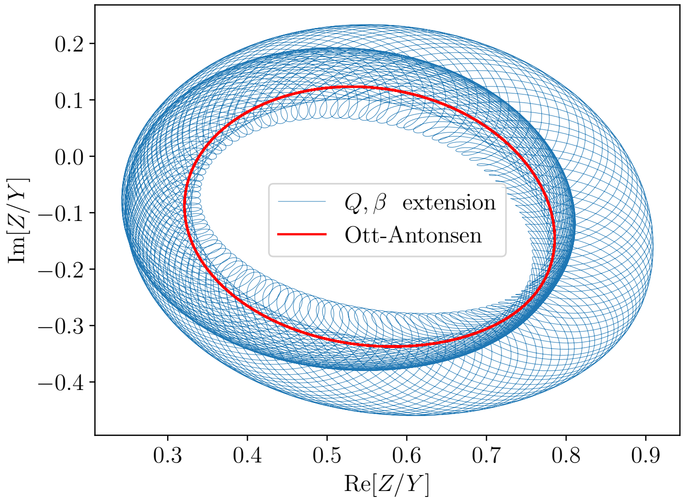


FIG. S3. Chimera state simulation in system (S14). Comparison of evolution on the Ott-Antonsen manifold (bold red line), to the evolution on the simplest $Q, \beta$ extended manifold with Eqs. (S15) (thin blue line).

### Addition of Gaussian white noise

Let us consider whether the exact invariant manifolds survive the addition of independent Gaussian white noise terms to the dynamics of the phases (as mentioned in the main text, for Cauchy white noise the invariant manifolds remain valid). In the phase equations noise enters as:

$$\dot{\varphi}_n = \omega(t) + \mathrm{Im}\big[2h(t)e^{-\mathrm{i}\varphi_n}\big] + \sigma\xi_n(t) \; , \tag{S16}$$

where $\xi_n$ are independent Gaussian white noises: $\langle \xi_n(t)\rangle = 0$, $\langle \xi_n(t)\xi_m(t')\rangle = 2\delta_{n,m}\delta(t-t')$. The kinetic equation for the probability density function then gets a diffusion term and becomes a Fokker-Planck equation:

$$\frac{\partial}{\partial t}P + \frac{\partial}{\partial \varphi}\Big((\omega - \mathrm{i}he^{-\mathrm{i}\varphi} + \mathrm{i}h^* e^{\mathrm{i}\varphi})P\Big) = \sigma^2 \frac{\partial^2}{\partial \varphi^2}P \; . \tag{S17}$$

The dynamics of the moments (S1) get an additional dissipation term proportional to $\sim n^2$:

$$\frac{1}{n}\dot{Z}_n = \mathrm{i}\omega Z_n + hZ_{n-1} - h^* Z_{n+1} - \sigma^2 n Z_n \; . \tag{S18}$$

And finally, the dynamical equation for the generating function is perturbed as:

$$\frac{\partial}{\partial t}F = \mathrm{i}\omega k \frac{\partial}{\partial k}F + hkF - h^* k\frac{\partial^2}{\partial k^2}F - \sigma^2 k \frac{\partial}{\partial k}\big(k\frac{\partial}{\partial k}F\big) \; . \tag{S19}$$

The OA Ansatz $F = e^{kQ}$ no longer satisfies this PDE, and hence for the same reason neither does Ansatz 1: $F = \sum e^{kQ_m}$. Trying Ansatz 2: $F = e^{kQ}G$, we can write the PDE for function $G$:

$$\frac{\partial}{\partial t}G = [\mathrm{i}\omega k - 2h^* Qk]\frac{\partial}{\partial k}G - h^* k \frac{\partial^2}{\partial k^2}G - \sigma^2\Big(Q^2k^2G + [k + 2Qk^2]\frac{\partial}{\partial k}G + k^2\frac{\partial^2}{\partial k^2}G\Big) \; , \tag{S20}$$

and see that apart from a non-derivative $G$ term, we also get terms proportional to $k^2$ which prevent us from finding finite solutions. However, we can still write the set of equations with $\beta_r$ variables, they just represent a non-truncatable infinite set of equations:

$$\begin{aligned} \dot{Q} &= \mathrm{i}\omega Q + h - h^* Q^2 - \sigma^2 Q \; , \\ \frac{1}{r}\dot{\beta}_r &= \mathrm{i}\omega\beta_r - 2h^* Q\beta_r - h^*\beta_{r+1} - \sigma^2 r\beta_r - \sigma^2(r-1)\big[2Q\beta_{r-1} + Q^2\beta_{r-2}\big] \; . \end{aligned} \tag{S21}$$

Notice that the neat hierarchy of $\beta_r$ that previously allowed us to truncate the system is now broken. Each $\beta_r$ equation (except $\beta_1$) gets additional terms proportional to $\beta_{r-1}$ and $\beta_{r-2}$. This means that the equation for $\beta_2$ contains a driving term $\sim Q^2$, and therefore in the presence of Gaussian noise, all the $Q, \beta_r$ variables are in general non-zero: an exact truncation is not possible. However, truncations will still approximate the dynamics. Typically the variables follow the ordering $\beta_{2r}, \beta_{2r-1} \sim \sigma^{2r}$ and thus truncating the system (S21) by considering just its first $2R$ equations results in an approximation of order $\mathcal{O}(\sigma^{2(R+1)})$, see section below for detailed argumentation.

### Gaussian noise approximation

Here we estimate the size scaling of our dynamical variables $Q, \beta_r$ in the case of weak Gaussian noise, and then estimate the order of approximation resulting from truncating system (S21). The argumentation is similar to that of [1]. Suppose the system contains either Cauchy-Lorentzian white noise or a Cauchy-Lorentzian distribution of frequencies which result in macroscopic dissipative terms: $-\gamma Q, -\gamma\beta_r$. Then, for weak Gaussian noise, $\sigma \ll 1$, the variables $\beta_r$ tend towards an established size ordering. Because of dissipation, the driving terms determine the size of variables. We consider $Q$ and $h$ to be the only macroscopic variables $\mathcal{O}(Q, h) \sim 1$ and assume that size of variables decreases with index $r$: $\mathcal{O}(\beta_{r+1}) \leq \mathcal{O}(\beta_r)$. Starting with $\beta_2$, it contains a driving term $\sim \sigma^2 Q^2$, so we conclude that it is of order $\beta_2 \sim \sigma^2$. Then, $\beta_2$ directly drives $\beta_1$ so it too is of order $\beta_1 \sim \sigma^2$, while it also drives both $\beta_3$ and $\beta_4$ with a prefactor $\sigma^2$ and hence they are of order $\beta_3, \beta_4 \sim \sigma^4$. $\beta_4$ then in turn drives $\beta_5$ and $\beta_6$ with a prefactor $\sigma^2$ and so they are of order $\beta_5, \beta_6 \sim \sigma^6$. By continuing this reasoning we can conclude that the ordering is: $\beta_{2r}, \beta_{2r-1} \sim \sigma^{2r}$ and thus, truncating system (S21) at $2R$ equations results in an approximation of order $\mathcal{O}(\sigma^{2(R+1)})$.

---

* rokcestn@uni-potsdam.de

[1] I. V. Tyulkina, D. S. Goldobin, L. S. Klimenko, and A. Pikovsky, Phys. Rev. Lett. **120**, 264101 (2018).
[2] I. V. Tyulkina, D. S. Goldobin, L. S. Klimenko, and A. Pikovsky, Radiophys. Quantum Electron. **61**, 640 (2019).
[3] S. Kato and M. C. Jones, Biometrika **102**, 181 (2014).
[4] D. M. Abrams, R. Mirollo, S. H. Strogatz, and D. A. Wiley, Phys. Rev. Lett. **101**, 084103 (2008).
[5] A. Pikovsky and M. Rosenblum, Phys. Rev. Lett. **101**, 264103 (2008).
[6] J. R. Engelbrecht and R. Mirollo, Phys. Rev. Research **2**, 023057 (2020).
[7] S. Watanabe and S. H. Strogatz, Phys. Rev. Lett. **70**, 2391 (1993).
